# Supplementary material for: Optical cycling in charged complexes with Ra-N bonds
Source: arXiv:2312.02732 ancillary file (2024-01-26)
Supplement: Supplementary file 1 [file supplementary.pdf]

# Supporting information for "Optical cycling in charged complexes with Ra–N bonds"

Timur Isaev, Alexander V. Oleynichenko, Dmitrii A. Makinskii, and Andrei Zaitsevskii
(Dated: January 26, 2024)

TABLE S1. Contracted Gaussian basis set for Ra ($s, p$ components)

```
s functions
exponents   contraction coefficients
14.89686    -0.1023458710  0.0169588248
11.45912     0.6649381916 -0.3329392095
6.9291713   -1.6638007361  1.0881900322
4.1267626    0.5982515243 -0.5867666495
2.4158729    0.5417656471 -0.3090581942
1.4153691    0.7484623420 -0.9772134517
0.84517663  -0.0737904640  0.3586520037
0.47543331   0.1060528486  0.4587255772
0.26884052  -0.0650850057  0.7270518427
0.14408405   0.0467898132  0.0201676541
0.088418964 -0.0301999942  0.0790788035
0.044870324  0.0137363228 -0.0353083378
0.024238512 -0.0072269440  0.0208304277
0.012957507  0.0027324581 -0.0080432569
0.006307096 -0.0005421761  0.0016346030
exponents    contraction coefficients
14.89686    -0.00325612  0.00052749 -0.01296040  0.03708847   0.04427306
11.45912     0.11094690  0.30474621 -0.46273376  0.86823436  -1.56950316
6.9291713   -0.38221751 -1.14087194  1.89764886 -4.10644799   7.82987562
4.1267626    0.21823033  0.67933247 -1.26475043  3.93146123 -13.09645582
2.4158729    0.10657704  0.54198162 -1.47967851  4.41637375   4.34509257
1.4153691    0.39820997  1.23340988 -0.82530622 -7.88305134  13.43165741
0.84517663  -0.17609424 -1.62877645  3.78723813 -0.68397928 -19.16408551
0.47543331  -0.25031226 -1.02117634 -0.08051138  7.29127860   7.96178299
0.26884052  -0.48899528  0.33442084 -2.40887735 -2.92760852   4.35184194
0.14408405  -0.18204908  0.63057268 -1.24140941 -2.94410574  -6.49158382
0.088418964  0.26689437  0.92560178  2.14439755  1.43675046   0.51960075
0.044870324  0.70404845  0.17897275  1.21785001  1.93255330   2.97054607
0.024238512  0.32605096 -0.99444928 -1.28759870 -1.07591323  -0.78083016
0.012957507  0.05976778 -0.17563446 -0.31162950 -0.27496962  -0.68090543
0.006307096 -0.00793202 -0.01285022 -0.00808887 -0.02172600   0.05295332
0.003069993  0.00336371  0.00483931  0.00290623  0.00853832  -0.02237156
0.001494326 -0.00083970 -0.00119787 -0.00076222 -0.00215618   0.00538617

p functions
exponents    contraction coefficients
8.92140     -0.2398133410 -0.8656491118   0.2271994801
7.43450      0.5974652582  3.6188162341  -0.5461565924
5.3424985   -0.0390263044 -4.1690098269   0.2229359843
3.04270432  -0.5152949395  0.6123639179   0.2169843620
1.71987993  -0.5174687836 -0.2323849238   0.4083559572
0.95405338  -0.2026719877  1.1098100489  -0.0150789134
0.50604988  -0.0084980830 -0.2303456128  -0.4170092957
0.26796428  -0.0097829931  0.2287207594  -0.5312113174
0.14281275   0.0057574028 -0.1452625059  -0.1994429253
0.072473572 -0.0036796586  0.0897008313  -0.0263157133
0.037058393  0.0023523648 -0.0565894489   0.0046799679
0.019107648 -0.0013496403  0.0323846505  -0.0032369217
0.009858256  0.0005992504 -0.0143234152   0.0013639971
0.004798528 -0.0001506950  0.0035960370  -0.0003464612
exponents    contraction coefficients
8.92140     -0.08141901  0.45773572 -0.51481174  0.83468486  1.87424271
7.43450      0.19222996 -1.08932994  1.23719656 -2.06699852 -4.96826855
5.3424985   -0.08171027  0.51044360 -0.57088198  0.94106524  3.86075163
3.04270432  -0.06926737  0.46094326 -0.79690220  2.17900860  2.33546948
1.71987993  -0.14377984  0.68448123 -0.32880535 -1.59246851 -6.55580221
0.95405338   0.02340307 -0.88623258  1.62715069 -2.14956620  4.62232489
0.50604988   0.17447969 -0.90065233 -0.11759618  3.20195640  0.77029348
0.26796428   0.22600620  0.43791880 -1.16236657 -0.35871259 -4.05273931
0.14281275   0.11674735  0.64280378 -0.15593037 -1.73612782  2.81552472
0.072473572 -0.25515579  0.32116123  0.96748980  0.45569657  0.41560464
0.037058393 -0.56204848 -0.16366779  0.55801302  1.22792770 -1.55915596
0.019107648 -0.31031937 -0.39637117 -0.83453579 -0.67046067  0.32831928
0.009858256 -0.05045713 -0.11336010 -0.30278132 -0.31668142  0.46901115
0.004798528 -0.00018562 -0.00047520 -0.00457700 -0.00809710 -0.00197618
```

TABLE S2. Contracted Gaussian basis set for Ra ($d-h$ components)

d functions

| exponents | contraction coefficients | | | | |
|---|---|---|---|---|---|
| 21.14549 | -0.00615760 | -0.02302189 | 0.00160390 | 0.00387791 | -0.00520144 |
| 6.91835 | -0.09586596 | -0.42630453 | 0.03560284 | 0.11213442 | -0.18578442 |
| 3.69372 | 0.22700949 | 1.74493511 | -0.09226919 | -0.31907073 | 0.62317086 |
| 2.0553207 | 0.45937275 | -0.76548908 | -0.13795439 | -0.39148343 | 0.55223711 |
| 1.1321279 | 0.33326702 | 0.14691579 | -0.11361451 | -0.07338506 | -1.02276035 |
| 0.60844286 | 0.13951891 | -0.76029003 | 0.14774156 | 0.76751914 | -0.36714746 |
| 0.26444538 | 0.01591998 | 0.07772885 | 0.31190957 | 0.39223903 | 0.81947645 |
| 0.12871939 | -0.00153915 | -0.11345388 | 0.31840953 | -0.28284893 | 0.19948582 |
| 0.06265445 | 0.00070684 | 0.07015484 | 0.32357702 | -0.27722451 | -0.17627588 |
| 0.03049720 | -0.00029127 | -0.03594243 | 0.15474588 | -0.22542085 | -0.42104995 |
| 0.01484458 | 0.00008400 | 0.01138743 | 0.03718874 | -0.03827956 | -0.11420283 |
| 0.00722563 | 0. | 0. | -0.00034954 | -0.00418367 | -0.00574367 |

| exponents | contraction coefficients | | |
|---|---|---|---|
| 21.14549 | 0.00537656 | -0.01197353 | 0.06997275 |
| 6.91835 | 0.24079343 | -0.46986485 | 0.16084163 |
| 3.69372 | -0.98123734 | 2.58718681 | -3.07426871 |
| 2.0553207 | -0.09948215 | -2.86112066 | 6.49145210 |
| 1.1321279 | 1.69269848 | 0.16412521 | -6.88232748 |
| 0.60844286 | -1.07587871 | 1.95678673 | 4.10142528 |
| 0.26444538 | -0.68216013 | -1.97900040 | -1.08818007 |
| 0.12871939 | 1.08905248 | 0.69207371 | -0.76486777 |
| 0.06265445 | 0.12841876 | 0.59602561 | 1.33160242 |
| 0.03049720 | -0.54670108 | -0.38428787 | -0.44461137 |
| 0.01484458 | -0.27649546 | -0.27342634 | -0.26385930 |
| 0.00722563 | 0.00578881 | 0.00279240 | -0.03454216 |

f functions

| exponents | contraction coefficients | | | | | |
|---|---|---|---|---|---|---|
| 21.623484 | -0.00029195 | 0.00073271 | 0.00560688 | 0.01467581 | 0.00509694 | -0.09178111 |
| 10.783703 | 0.02032622 | 0.01312922 | -0.02212772 | -0.07252745 | -0.08616712 | 0.75063633 |
| 6.9241349 | -0.02564398 | 0.00042890 | 0.09376404 | 0.26879697 | 0.01530867 | -1.54569729 |
| 3.8201017 | -0.16693101 | -0.24465722 | -0.46335044 | -1.17557701 | 1.41988976 | 0.38976485 |
| 1.9946900 | -0.51470582 | -0.52767320 | -0.12777882 | 0.70905206 | -1.84253161 | 0.94393112 |
| 0.7761069 | -0.40282004 | 0.36318453 | 0.81942767 | 0.72079418 | 1.12798356 | -1.90583014 |
| 0.3715763 | -0.08042193 | 0.55825534 | -0.20698606 | -1.21639369 | -0.07579609 | 2.60372813 |
| 0.1808656 | -0.05769966 | 0.09728984 | -0.42604910 | 0.33940628 | -0.90438140 | -2.07113675 |
| 0.0880367 | 0.01109267 | 0.08461493 | -0.32741031 | 0.23740134 | 0.45922898 | 0.56728927 |
| 0.0428521 | -0.01234463 | 0.00706286 | -0.15767567 | 0.36149423 | 0.30414964 | 0.19615654 |
| 0.0208583 | 0.00255766 | 0.00899809 | -0.02972681 | 0.02387395 | 0.10564551 | 0.19884484 |

g functions

| exponents | contraction coefficients | | | |
|---|---|---|---|---|
| 6.573264 | -0.057949264 | 0.107895965 | 0.140597527 | 0.270162718 |
| 3.5527187 | -0.135154016 | 0.410140713 | 0.678584108 | 0.711178524 |
| 1.9201739 | -0.303107430 | 0.459352085 | -0.239676415 | -1.271378069 |
| 1.0365027 | -0.286410451 | -0.072550728 | -0.965532174 | 0.161390808 |
| 0.6343499 | -0.372538587 | -0.542928624 | 0.450851607 | 0.795677993 |
| 0.27741068 | -0.127069042 | -0.246851659 | 0.493344800 | -0.377168844 |
| 0.12131583 | -0.000880360 | -0.015657957 | 0.176943330 | -0.544037910 |

h functions

| exponents | contraction coefficients | | |
|---|---|---|---|
| 5.923926 | 0.06673968 | -0.12821497 | -0.3828683 |
| 2.961963 | 0.31204863 | -0.65095417 | -0.5806803 |
| 1.480982 | 0.43835172 | -0.07760140 | 1.1227287 |
| 0.740491 | 0.36746181 | 0.63450668 | -0.2752368 |
| 0.3702454 | 0.07535442 | 0.21078077 | -0.4838897 |
| 0.1851227 | 0.01518463 | 0.04451950 | -0.1362951 |

TABLE S3. Frozen ligand geometry parameters assumed in large-scale calculations of complexes with $Ra^+$.

| Ligand | Symmetry | Geometry |
|---|---|---|
| NCH | $C_{\infty v}$ | R(N-C) = 1.150 Å |
| | | R(C-H) = 1.070 Å |
| $NH_3$ | $C_{3v}$ | R(N-H) = 1.017 Å |
| | | ∠ RaNH = 113.43° |
| | | ∠ HNH = 105.24° |
| $NCCH_3$ | $C_{3v}$ | R(N-C) = 1.157 Å |
| | | R(C-C) = 1.438 Å |
| | | R(C-H) = 1.113 Å |
| | | ∠ CCH = 108.94° |

TABLE S4. FS RCCSD / CCSD(T) total energies (a.u.) of low-lying electronic states of symmetric ($C_{\infty v}$) $RaNCH^+$ ion as functions of the Ra–N internuclear separation (a.u.)

| $r$(Ra–N) | $X$(1)1/2 | (1)3/2 | (2)1/2 | (2)3/2 | (1)5/2 |
|---|---|---|---|---|---|
| 5.0443 | -437.352554122991 | -437.303028462679 | -437.303695525387 | -437.297722229385 | -437.294084914740 |
| 5.2443 | -437.354796316454 | -437.303909970910 | -437.303343567441 | -437.298644032168 | -437.296416604437 |
| 5.4443 | -437.355504123846 | -437.304073616705 | -437.302307705018 | -437.297918107195 | -437.297087588451 |
| 5.6443 | -437.355214973208 | -437.303468895629 | -437.300839039561 | -437.296430119023 | -437.296664596864 |
| 5.8443 | -437.354303485328 | -437.302290147095 | -437.299113767940 | -437.294573222695 | -437.295547254081 |
| 6.0443 | -437.353838351461 | -437.301559085707 | -437.298072717417 | -437.293361749255 | -437.294825620890 |

TABLE S5. FS RCCSD / CCSD(T) total energies (a.u.) of low-lying electronic states of symmetric ($C_{3v}$) $RaNH_3^+$ ion as functions of the Ra–N internuclear separation (a.u.)

| $r$(Ra–N) | $X(1)E_{1/2}$ | $(1)E_{3/2}$ | $(2)E_{1/2}$ | $(3)E_{1/2}$ | $(2)E_{3/2}$ |
|---|---|---|---|---|---|
| 5.027293 | -400.552273136 | -400.498275482 | -400.492650325 | -400.488508423 | -400.485014850 |
| 5.227293 | -400.554815063 | -400.501283330 | -400.495497165 | -400.492695658 | -400.489032417 |
| 5.427293 | -400.555678087 | -400.502462316 | -400.496533714 | -400.494767244 | -400.490932944 |
| 5.627293 | -400.555413328 | -400.502385960 | -400.496336003 | -400.495374769 | -400.491373712 |
| 5.827293 | -400.554414880 | -400.501471427 | -400.495343108 | -400.494972147 | -400.490833577 |
| 6.027293 | -400.552961781 | -400.500019538 | -400.494075874 | -400.493682157 | -400.489658106 |
| 6.227293 | -400.551249896 | -400.498245717 | -400.492654128 | -400.491845441 | -400.488094754 |

TABLE S6. FS RCCSD / CCSD(T) total energies (a.u.) of low-lying electronic states of symmetric ($C_{3v}$) $RaNCCH_3^+$ ion as functions of the Ra–N internuclear separation (a.u.)

| $r$(Ra–N) | $X(1)E_{1/2}$ | $(1)E_{3/2}$ | $(2)E_{1/2}$ | $(3)E_{1/2}$ | $(2)E_{3/2}$ |
|---|---|---|---|---|---|
| 4.8892 | -476.623040543 | -476.570845660 | -476.570383156 | -476.565914048 | -476.563613976 |
| 5.0892 | -476.626048231 | -476.573502253 | -476.571551753 | -476.567520307 | -476.566898512 |
| 5.2892 | -476.627054555 | -476.574455503 | -476.571409988 | -476.568032771 | -476.567346911 |
| 5.4892 | -476.626742799 | -476.574115215 | -476.570380559 | -476.567731962 | -476.566147147 |
| 5.6892 | -476.625597625 | -476.572905956 | -476.568778715 | -476.566507592 | -476.564337192 |
| 5.8892 | -476.623954851 | -476.571155490 | -476.566837338 | -476.564718146 | -476.562185092 |
